# Supplementary material for: On the Intrinsic and Extrinsic Fairness Evaluation Metrics for Contextualized Language Representations
Source: arXiv:2203.13928 source file (2022-03-25)
Supplement: Supplementary file 1 [file supplement.tex]

% This must be in the first 5 lines to tell arXiv to use pdfLaTeX, which is strongly recommended.
\pdfoutput=1
% In particular, the hyperref package requires pdfLaTeX in order to break URLs across lines.

\documentclass[11pt]{article}

% Remove the "review" option to generate the final version.
\usepackage[review]{acl}

% Standard package includes
\usepackage{times}
\usepackage{graphicx}
\usepackage{latexsym}
\usepackage{array}
\usepackage{multirow, booktabs}
% For proper rendering and hyphenation of words containing Latin characters (including in bib files)
\usepackage[T1]{fontenc}
% For Vietnamese characters
% \usepackage[T5]{fontenc}
% See https://www.latex-project.org/help/documentation/encguide.pdf for other character sets

% This assumes your files are encoded as UTF8
\usepackage[utf8]{inputenc}

% This is not strictly necessary, and may be commented out,
% but it will improve the layout of the manuscript,
% and will typically save some space.
\usepackage{microtype}

% trista format ---------------

\definecolor{darkergreen}{rgb}{0.0,0.4,0.0}

\usepackage{xspace}

\usepackage{siunitx}

\title{On the Intrinsic and Extrinsic Bias Evaluation Metrics \\for Contextualized Language Representations\\ - Supplementary Material}

\date{}

\begin{document}
\maketitle

\section{Target Category Term Substitutions}
\end{document}
